# Supplementary material for: Graph Matching via convex relaxation to the simplex
Source: arXiv:2310.20609 source file (2024-08-09)
Supplement: Supplementary file 1 [file previous_results_appendix.tex]

%Pop. Dynamics corollary, that follows from the main results. PSD approach... 
In a similar spirit, we have the following result, whose proof can be found in Appendix \ref{app:proofs}.
%Cor. 
\begin{corollary}\label{cor:pd_iter_population}
Suppose $\sigma \leq 1$. If the sequence of learning rates $(\gamma_k)^N_{k=0}\in\matR_+$ satisfies \eqref{eq:condition_rates}, for a given $N\in\matN$, then all the iterates $\Xk$, up to $N$, of the population dynamics defined by \eqref{eq:pop_dyn_init} and \eqref{eq:pop_dyn_update} satisfy the following:
\begin{enumerate}[label=(\roman*)]
    \item $\Xk$ satisfy \eqref{eq:Xk_pop_dyn} and, in addition, we have $0<\frac12 \Xk_{11}<\Xk_{12}<\Xk_{11}$, for all $k\in [N]$.
    \item The $\Xk$ are positive definite for all $k\in [N]$.
\end{enumerate}
\end{corollary}
\begin{proof}[Proof of Corollary \ref{cor:pd_iter_population}]
    The first assertion in $(i)$ follows from Lemma \ref{lem:Xk_pop_dyn}. The second assertion of $(i)$ was already proven as an intermediate step in the proof of Proposition \ref{prop:pop_dyn_multistep}. Indeed, there we proved that $\frac12<r_k<1$, which is clearly equivalent to the statement of $(i)$. 
    
    To prove $(ii)$, we argue by induction. Inspecting the proof of Proposition \ref{prop:noiseless_dyn_onestep}, we see that $\Xone$ is a positive scalar times the matrix $J+(e^{2\frac{\gamma_0}{n^2}}-1)\id$. For $\gamma_0>0$ we have that $(e^{2\frac{\gamma_0}{n^2}}-1)\id$ is positive definite and given that $J$ is positive semidefinite, we conclude that $J+(e^{2\frac{\gamma_0}{n^2}}-1)\id$ is positive definite. Now, we assume that $\Xk$ is positive definite. We have that $\Xkone$ is a positive scalar times the matrix $\Xk\odot e^{-\gamma_k\popgradient (\Xk)}$. If we can prove that $e^{-\gamma_k\popgradient(\Xk)}$ is positive definite, then by virtue of the Schur product theorem  we will obtain that $\Xkone$ is positive definite, finishing the proof. We now prove that $e^{-\gamma_k\popgradient(\Xk)}$ positive definite. For that we will use Theorem \ref{thm:condp_to_exppd}. To verify that the hypothesis of Theorem \ref{thm:condp_to_exppd} hold we take $u\in \matR^{n}$ such that $\ones^Tu=0$. We have
    \begin{align*}
    -u^T\popgradient (\Xk)u&=-(2+\sigma)\frac{n+1}{n}u^T\Xk u+\frac2n\Tr(\Xk)u^Tu +\frac2nu^T{\Xk}^T u\\
    &=-(2+\sigma\frac{n+1}{n})u^T\Xk u+\frac2n\Tr(\Xk)\|u\|^2_2\\
    &=-(2+\sigma\frac{n+1}{n})\big(\Xk_{11}\|u\|^2_2+\Xk_{12}\sum_{i\neq j}u_iu_j\big)+2\Xk_{11}\|u\|^2_2\\
    &=(2+\sigma\frac{n+1}{n})\Xk_{12}\|u\|^2_2-\sigma\frac{n+1}{n}\Xk_{11}\|u\|^2_2,
    \end{align*}
    where in the second equality we used the fact that $\Xk$ is symmetric, in the third equality we used Lemma \ref{lem:Xk_pop_dyn} and in the fourth equality we used the fact that $0=\sum^n_{i=1}\sum^n_{j=1}u_iu_j=\|u\|^2_2+\sum_{i\neq j}u_iu_j$. By Proposition \ref{prop:pop_dyn_multistep}, given that the rates satisfy \eqref{eq:condition_rates}, we have that $r_k<1$ for all $2\leq k\leq N$ or, equivalently, $a_\sigma\Xk_{12}-(a_\sigma-2)\Xk_{11}>0$, which clearly implies that $-u^T\popgradient (\Xk)u>0$. Then the matrix $\popgradient(\Xk)$ is conditionally positive definite, and trivially the same is true for $\gamma_k\popgradient(\Xk)$, then by Theorem \ref{thm:condp_to_exppd} we obtain that $e^{-\gamma_k\popgradient(\Xk)}$ is positive definite, which completes the proof.
\end{proof}
